# Supplementary material for: Topology-Aware Hashing for Effective Control Flow Graph Similarity Analysis
Source: arXiv:2004.06563 source file (2020-04-14)
Supplement: Supplementary file 1 [file appendix.tex]

\section{Appendix}
\appendix 

%\section{CFG algorithm optimal clustering results}

\begin{table*}[h]
\caption{Optimal clustering results for different algorithms}
\label{table:cfg_clustering}
\centering
\scalebox{0.9}{
\begin{tabular}{|c||c|c|c|c||c|c|c|c|}
  \hline
  \multirow{2}{*}{Algorithm} & \multicolumn{4}{c||}{{\bf CFG20-1} Dataset} & \multicolumn{4}{c|}{{\bf CFG20-3} Datase} \\ \cline{2-9}
  & {Single } &  {Average} &  {Complete} & {Avg F-score} & {Single} &  {Average} &  {Complete} & {Avg F-score} \\
%  & linkage & linkage & linkage & F-score & linkage & linkage & linkage & F-score \\ 
% & {Opt {\it d}} & {F-score}& {Opt {\it d}} & {F-score}& {Opt {\it d}} & {F-score} \\
\hline
\hline
Hu & 0.847 & 0.872 & 0.879 & 0.866 & 0.634 & 0.812 & 0.794 & 0.747 \\
Vujošević & 0.749 & 0.869 & 0.876 & 0.831 & 0.617 & 0.791 & 0.764 & 0.724 \\
Sokolsky & 0.367 & 0.456 & 0.501 & 0.441 & 0.407 & 0.431 & 0.435 & 0.424 \\
Kruegel & 0.530 & 0.530 & 0.530 & 0.530 & 0.462 & 0.462 & 0.462 & 0.462\\
McGreger & 0.597 & 0.588 & 0.324 & 0.503 & 0.398 & 0.608 & 0.284 & 0.430 \\
\algoname & 0.816 & 0.926 & 1.000 & 0.914 & 0.597 & 0.747 & 0.804 & 0.716 \\
\fuzzname & 0.817 & 0.926 & 0.864 & 0.869 & 0.596 & 0.669 & 0.581 & 0.615 \\
\hline
\end{tabular}
}
\end{table*}

%\section{CFG algorithm different output ranges}

\begin{table*}[h]
\caption{Distance ranges for different CFG pairs}
\label{table:distance}
\centering
\scalebox{0.9}{
\begin{tabular}{|c||c|c|c|c|c|c||c|c|c|c|c|c|}
\hline
  \multirow{3}{*}{Algorithm} & \multicolumn{6}{c||}{{\bf CFG20-1} Dataset} &  \multicolumn{6}{c|}{{\bf CFG20-3} Dataset} \\ \cline{2-13}
& \multicolumn{2}{c|}{Same-group} & \multicolumn{2}{c|}{Diff-group} & \multicolumn{2}{c||}{All pairs} & \multicolumn{2}{c|}{Same-group} & \multicolumn{2}{c|}{Diff-group} & \multicolumn{2}{c|}{All groups}\\ \cline{2-13}
& {   Min   } & {   Max   }& {   Min   } & {   Max   }& {   Min   } & {   Max   } & {   Min   } & {   Max   }& {   Min   } & {   Max   }& {   Min   } & {   Max   } \\
\hline
\hline
Hu & 0.000 & 0.049 & 0.000 & 0.182 & 0.000 & 0.182 & 0.000 & 0.032 & 0.029 & 0.165 & 0.000 & 0.165 \\
Vujošević & 0.000 & 0.100 & 0.000 & 0.213 & 0.000 & 0.213 & 0.000 & 0.067 & 0.028 & 0.203 & 0.000 & 0.203 \\
Sokolsky & 0.000 & 0.258 & 0.000 & 0.258 & 0.000 & 0.258 & 0.000 & 0.250 & 0.000 & 0.250 & 0.000 & 0.250 \\
Kruegel & 0.000 & 1.000 & 0.000 & 1.000 & 0.000 & 1.000 & 0.000 & 1.000 & 0.000 & 1.000 & 0.000 & 1.000 \\
McGreger & 0.000 & 0.905 & 0.000 & 0.800 & 0.000 & 0.905 & 0.000 & 0.935 & 0.000 & 0.833 & 0.000 & 0.935 \\
CFGSimNG & 0.007 & 0.724 & 0.181 & 0.921 & 0.007 & 0.921 & 0.000 & 0.777 & 0.294 & 0.917 & 0.000 & 0.917 \\
CFGSimNG\_H & 0.015 & 0.978 & 0.328 & 1.000 & 0.015 & 1.000 & 0.000 & 0.964 & 0.398 & 1.000 & 0.000 & 1.000 \\
\hline
\end{tabular}
}
\end{table*}

%\section{Detailed CFG Clustering Results}

\begin{figure*}[ht]
  \centering
  \includegraphics[width=\linewidth,height=.3\textheight]{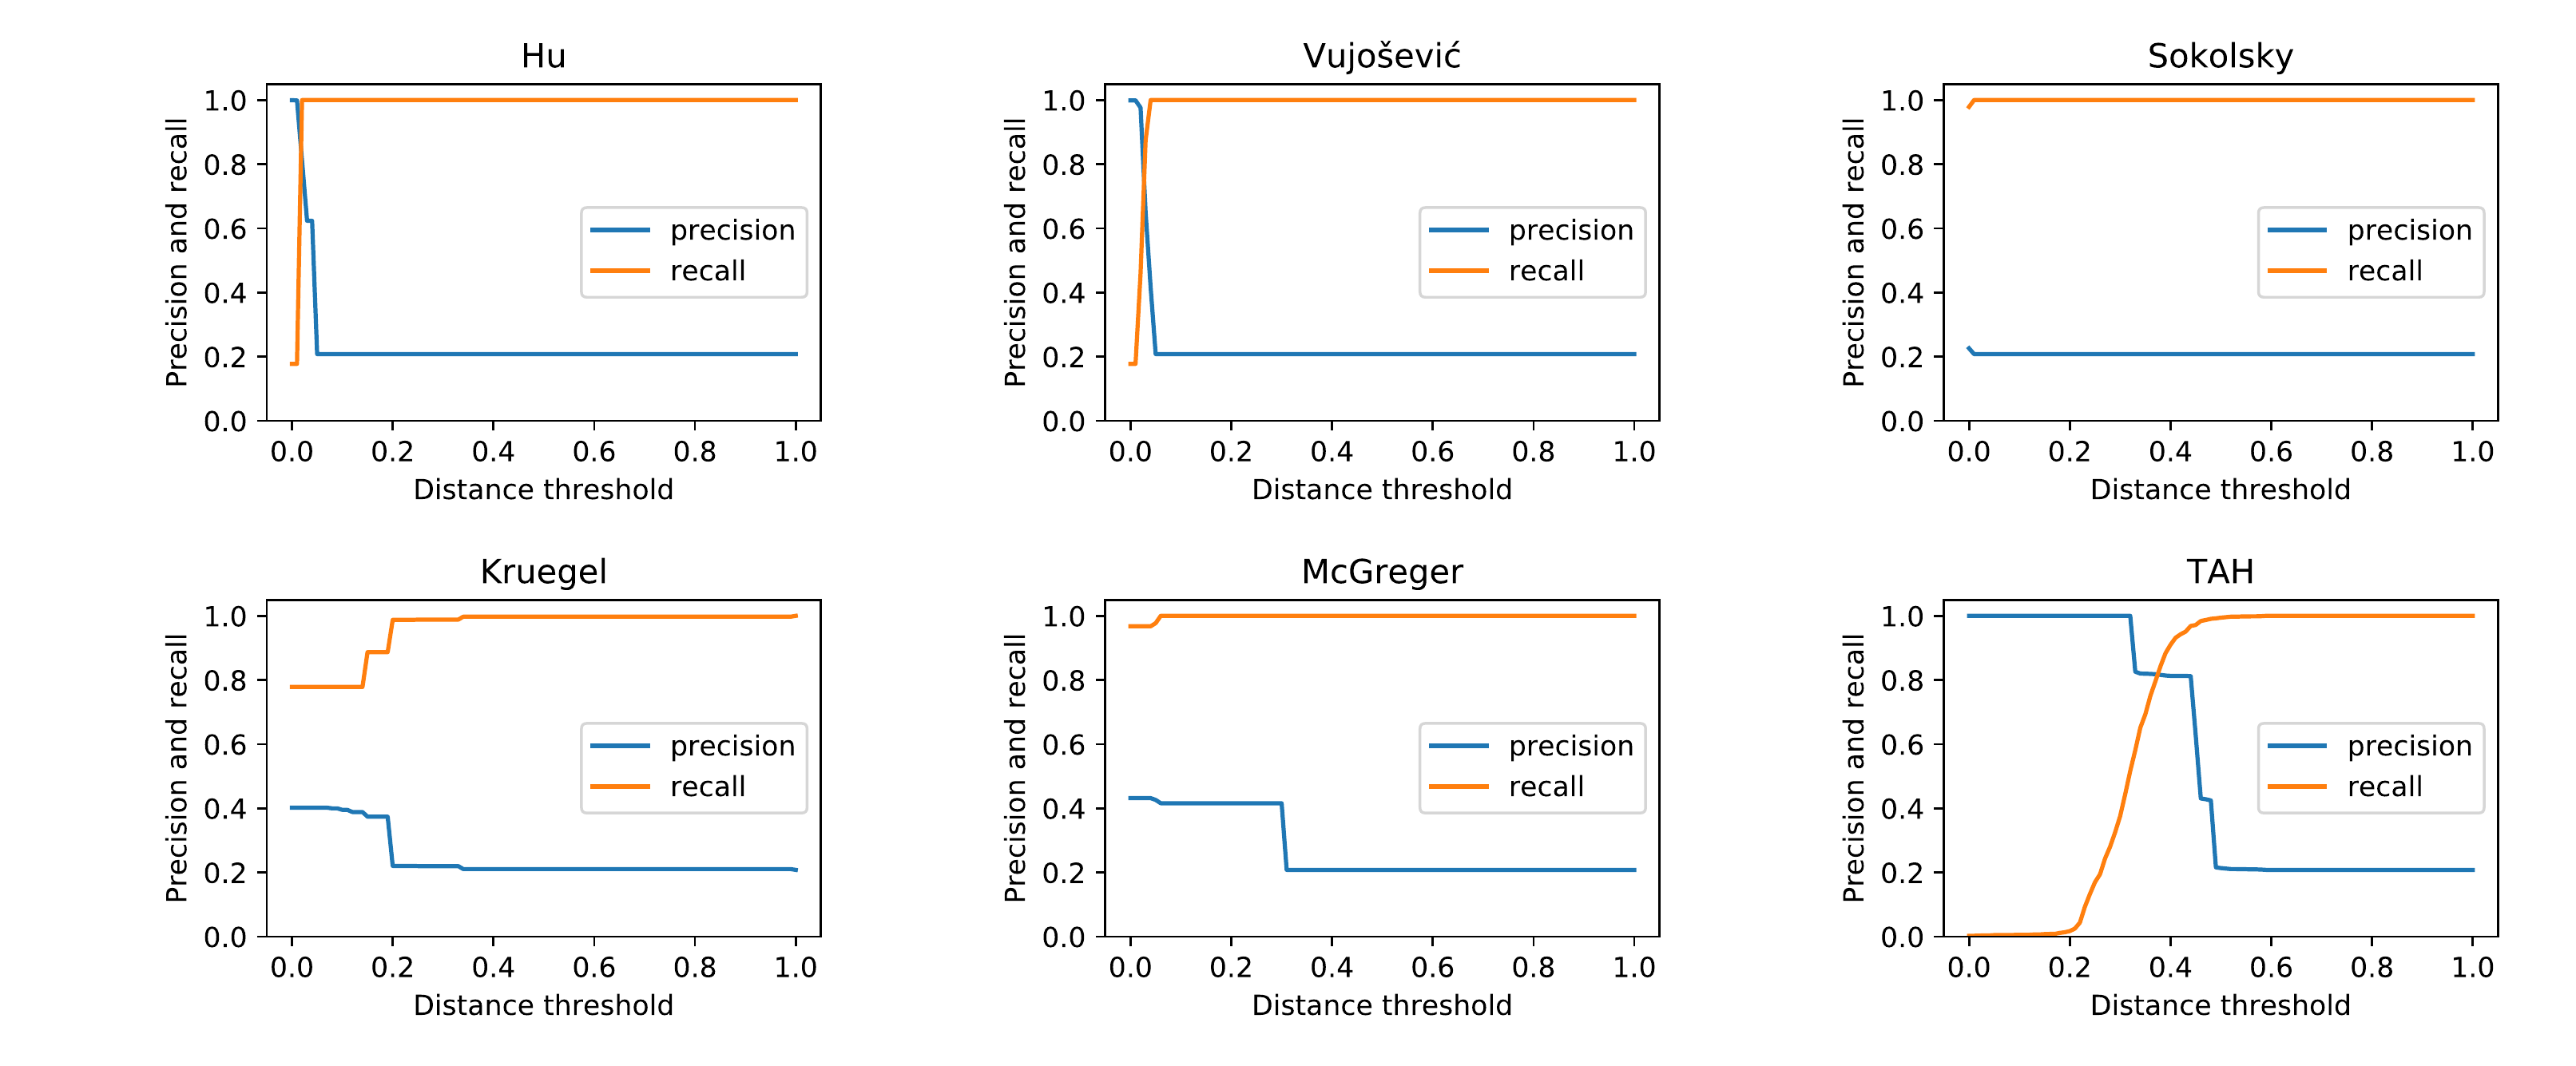}
  \centering
  \caption{Single-linkage clustering results for different CFG comparison algorithms}
  \label{fig:sim_res1}
\end{figure*}

% \begin{figure*}[ht]
%   \centering
%   \includegraphics[width=\linewidth,height=.3\textheight]{images/average_cluster_results}
%   \centering
%   \caption{Average-linkage clustering results for different CFG comparison algorithms}
%   \label{fig:sim_res2}
% \end{figure*}

% \begin{figure*}[ht]
%   \centering
%   \includegraphics[width=\linewidth,height=.3\textheight]{images/complete_cluster_results}
%   \centering
%   \caption{Complete-linkage clustering results for different CFG comparison algorithms}
%   \label{fig:sim_res3}
% \end{figure*}

% Figure generation params:
% left: 0.10
% bottom: 0.12
% right: 0.97
% top: 0.92
% wspace: 0.51
% hspace: 0.53

% \begin{figure*}[!htb]
%     \centering
%    \begin{subfigure}[b]{\textwidth}
%         \centering
%         \includegraphics[width=\linewidth]{images/single_cluster_results}
%         \caption{Single-linkage clustering results}
%         \label{fig:sim_res1}
%     \end{subfigure}\hfill %
%     \begin{subfigure}{\textwidth}
%         \centering
%         \includegraphics[width=\linewidth]{images/average_cluster_results}
%         \caption{Average-linkage clustering results}
%         \label{fig:sim_res2}
%     \end{subfigure}\hfill %
%     \begin{subfigure}{\textwidth}
%         \centering
%         \includegraphics[width=\linewidth]{images/complete_cluster_results}
%         \caption{Complete-linkage clustering results}
%         \label{fig:sim_res3}
%     \end{subfigure}
%     \caption{Evaluation results for different CFG comparison algorithms}
%     \label{fig:sim_res}
% \end{figure*}

%%% Local Variables:
%%% mode: latex
%%% TeX-master: "paper"
%%% End:
